# Supplementary material for: Seeing Around Corners with Edge-Resolved Transient Imaging
Source: arXiv:2002.07118 source file (2020-02-17)
Supplement: Supplementary file 1 [file notation.tex]

% For comments
  % an "inert" form of \frac

% Vectors

% Matrices

% Transpose 

%%%%%%%%%%%%%%%%%%%%%%%%%%%%%%%%%%%%

     % Like \mid, but with less space; use for conditioning
  % Make it easier to parse many expressions with \sim
